# Supplementary material for: CaRaFFusion: Improving 2D Semantic Segmentation with Camera-Radar Point Cloud Fusion and Zero-Shot Image Inpainting
Source: arXiv:2505.03679 source file (2025-05-06)
Supplement: Supplementary file 1 [file X_suppl.tex]

\clearpage
\setcounter{page}{1}
\maketitlesupplementary

\section{Inpainting Details}
\label{sec:inpainting_details}
In order to generate high-quality and realistic inpainted images, one should choose the guidance scale and the inference steps carefully. During inference, the guidance scale amplifies the influence of the conditioning signal compared to the model’s original predictions for unconditional generation. Low guidance scale leads to more creative outputs, but it might lack realism for our use case. If it is too high, the generated image might be overfitted to the prompt. In our case, we choose the guidance scale as \textbf{7} based on our experimental approach. In order to reduce the noise properly, we select the number of inference steps as \textbf{50} which is enough to reconstruct the rest of the image content and inpainted part of the object. 

\subsection{Inpainted Images}

As the generated masks are not perfect, this also leads to non-perfect objects during the generative process. In this subsection, we give some examples:

\begin{figure}[h]
    \centering
    \includegraphics[width=0.4\linewidth]{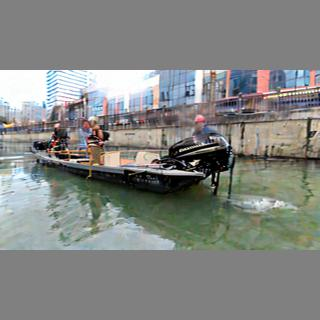}
    \caption{Mislocated radar points can lead to the generation of objects at wrong locations. In this example, a person is generated where he should not be.}
    \label{fig:1}
\end{figure}

\begin{figure}[h]
    \centering
    \includegraphics[width=0.4\linewidth]{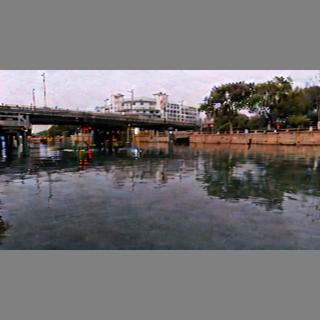}
    \caption{Radar cluttter can cause noisy artefacts in the generated image. In this example, red areas around the bridge must not be generated.}
    \label{fig:3}
\end{figure}

\begin{figure}[h]
    \centering
    \includegraphics[width=0.4\linewidth]{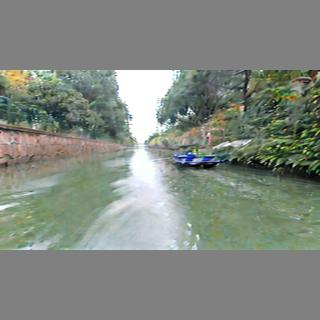}
    \caption{Wrongly generated images can lead to lost objects that have to be segmented.}
    \label{fig:3}
\end{figure}

\begin{figure}[h]
    \centering
    \includegraphics[width=0.4\linewidth]{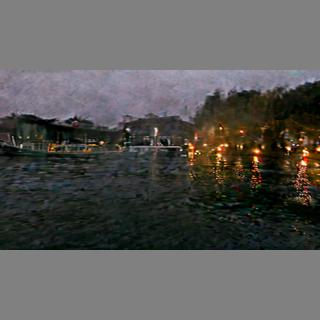}
    \caption{An example where the generated image is corrupted due to the generation process.}
    \label{fig:3}
\end{figure}

\begin{figure}[h]
    \centering
    \includegraphics[width=0.4\linewidth]{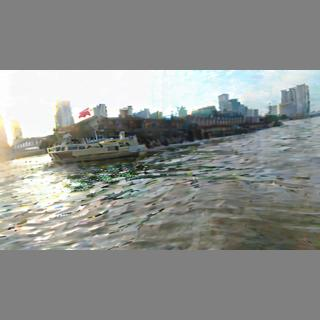}
    \caption{Generated images can contain changed object textures. }
    \label{fig:3}
\end{figure}
